# Supplementary material for: Impact of Data Quality on Renewable Energy Potential Estimations
Source: arXiv:2204.02334 ancillary file (2022-04-05)
Supplement: Supplementary file 1 [file Supplementary.pdf]

# Impact of Data Quality on Renewable Energy Potential Estimations (Supplementary Material)

Stanley Risch, Rachel Maier, Junsong Du, Noah Pflugradt, Peter Stenzel, Leander Kotzur and Detlef Stolten

## General Feature Definition

**Table 1**
Feature definition. Filename is given if different files are applied for one dataset.

| Criterion | Dataset | Filename / Query | Filter or code |
|---|---|---|---|
| **Lake** | Basis-DLM [1] | ver04_f | OBJART_TXT='AX_Hafenbecken' OR OBJART_TXT='AX_StehendesGewaesser' |
| | OSM [2] retrieved from Geofabrik [3] | gis_osm_transport_a_free_1 | fclass not in (’river’,’riverbank’,’drain’,’canal’,’tidal_channel’) |
| | CLC [4] | | Code_18 in (’512’,’521’) |
| **River** | Basis-DLM [1] | gew01_f | OBJART_TXT='AX_Fliessgewaesser' OR OBJART_TXT='AX_Kanal' OR OBJART_TXT='AX_Wasserlauf' OR OBJART_TXT='AX_Gewaesserachse' |
| | OSM [2] retrieved from Geofabrik [3] | gis_osm_water_a_free_1 | fclass='river' OR fclass='drain' OR fclass='canal' OR fclass='tidal_channel' OR fclass='riverbank' |
| | CLC [4] | | Code_18 in (’511’,’522’) |
| **Stream** | OSM [2] retrieved from Geofabrik [3] | gis_osm_waterways_free_1 | fclass='stream' OR fclass='ditch' |
| **Motorway** | Basis-DLM [1] | ver01_l | WDM = ’1301’ |
| | | ver01_f | OBJART_TXT = 'AX_Platz' and FKT != '5310' |
| | OSM [2] retrieved from Geofabrik [3] | gis_osm_roads_free_1 | fclass in (’motorway’,’motorway_link’) |
| **Primary roads** | Basis-DLM [1] | ver01_l | WDM = ’1303’ |
| | OSM [2] retrieved from Geofabrik [3] | gis_osm_roads_free_1 | fclass in (’primary’,’primary_link’) |
| **Secondary roads** | Basis-DLM [1] | ver01_l | WDM = '1305' |
| | OSM [2] retrieved from Geofabrik [3] | gis_osm_roads_free_1 | fclass in (’secondary’, ’secondary_link’) |

| | | | |
|---|---|---|---|
| **Regional roads** | Basis-DLM [1] | ver01_l | WDM != '1301' AND WDM != '1303' AND WDM != '1305' |
| | OSM [2] retrieved from Geofabrik [3] | gis_osm_roads_free_1 | fclass = ('residential', 'tertiary', ’tertiary_link') |
| **Railways** | Basis-DLM [1] | ver03_l | OBJART_TXT = 'AX_Bahnstrecke' |
| | | ver03_f | None |
| | | ver06_f | OBJART_TXT = 'AX_Bahnverkehrsanlage' |
| | OSM [2] retrieved from Geofabrik [3] | gis_osm_railways_free_1 | None |
| **Power lines** | Basis-DLM [1] | sie03_l | OBJART_TXT='AX_Leitung' |
| | OSM [2] retrieved from Overpass-Turbo [5] (query on the right) | [out:json] [timeout:250]; area[name="Deutschland"]->.searchArea; (way[power=line](area.searchArea);); (._;>;); out meta; | None |
| **Farmland** | Basis-DLM [1] | veg01_f | VEG != ’1020’ |
| | OSM [2] retrieved from Geofabrik [3] | gis_osm_landuse_a_free_1 | fclass=’farmland’ OR fclass=’orchard’ OR fclass=’vineyard’ |
| | CLC [4] | | Code_18 in ('211’,’212’,’213’, ‘221’,’222’,’223’, '241‘,‘242‘,‘243‘,‘244‘) |
| **Grassland** | Basis-DLM [1] | veg01_f | VEG = ’1020’ |
| | OSM [2] retrieved from Geofabrik [3] | gis_osm_landuse_a_free_1 | fclass=’grass’ OR fclass=’meadow’ |
| | CLC [4] | | Code_18=’231’ |
| **Forests** | Basis-DLM [1] | veg02_f | None |
| | OSM [2] retrieved from Geofabrik [3] | gis_osm_landuse_a_free_1 | fclass=’forest’ |
| | CLC [4] | | Code_18 in (’311’,’312’,’313’) |
| **Trees** | Basis-DLM [1] | veg03_f | OBJART_TXT = 'AX_Gehoelz' |
| **Residential** | Basis-DLM [1] | sie02_f | OBJART = '41001' OR (OBJART='41007' AND FKT in ('1110', '1120', '1130', '1150', '1160', '1170')) |
| | OSM [2] retrieved from Geofabrik [3] | gis_osm_landuse_a_free_1 | fclass='residential' OR fclass='retail' OR fclass='allotments' |
| | CLC [4] | | Code_18='111' OR Code_18='112' OR |

| | | | |
|---|---|---|---|
| | | | Code_18='133' OR Code_18='141' OR Code_18='142' |
| **Inner areas** | Basis-DLM [1] | sie01_f | None |
| **Outer areas** | Basis-DLM [1] | sie02_f | OBJART = '41001' OR (OBJART='41007' AND FKT in('1110', '1120', '1130', '1150', '1160', '1170') |
| **Buildings residential** | Hausumringe [6] | | GFK IN ('31001_1000', '31001_1010', '31001_1020', '31001_1021', '31001_1022', '31001_1023', '31001_1024', '31001_1025', '31001_1210', '31001_3064', '31001_3066', '31001_2070', '31001_2071', '31001_2072', '31001_2074') |
| **Buildings health treatment** | Hausumringe [6] | | GFK IN ('31001_3240', '31001_3241', '31001_3242', '31001_3051', '31001_3052') |
| **Buildings mixed** | Hausumringe [6] | | GFK IN ('31001_1100', '31001_1110', '31001_1120', '31001_1121', '31001_1122', '31001_1123', '31001_1130', '31001_1220', '31001_1221', '31001_1223') |
| **Buildings all** | Hausumringe [6] | | None |
| **Camping** | Basis-DLM [1] | sie02_f | FKT = '4330' |
| **Industrial/ Commercial** | Basis-DLM [1] | sie02_f | OBJART =’41002’ |
| | OSM [2] retrieved from Geofabrik [3] | gis_osm_landuse_a_free_1 | fclass in (’commercial’, ’industrial’) |
| | CLC [4] | | Code_18=’121’ |
| **VOR** | OSM [2] retrieved from Overpass-Turbo [5] (query on the right) | [out:json] [timeout:250]; area[name="Deutschland"]->.searchArea; (node[airmark=beacon](area.searchArea);); (._;>;); out meta; | "beacon_typ" in ( 'VOR', 'VOR-DME', 'VOR/DME', 'VOR;DME' , 'VOR;TACAN' ) or "type" in ( 'VOR/DME' ) or "beacon_t_1" in ('VOR', 'VOR;TACAN') |

| | | | |
|---|---|---|---|
| **D-VOR** | OSM [2] retrieved from Overpass-Turbo [5] (query on the right) | [out:json] [timeout:250]; area[name="Deutschland"]->.searchArea; (node[airmark=beacon](area.searchArea);); (._;>;); out meta; | "beacon_typ" in ( 'DVOR' ,'DVOR/DME' ,'DVOR;DME' ,'DVOR;TACAN' , 'DVORTAC' ) or "beacon_t_1" in ( 'DVOR' , 'DVOR-DME' , 'DVOR/DME' , 'DVOR;DME' ) |
| **Seismic station** | BGR [7] | | None |
| **Airports** | Basis-DLM [1] | ver04_f | ART in (’5510’,’5511’,’5512’) OR NTZ in (’2000’,’3000’) AND ZUS IS NULL |
| | OSM [2] retrieved from Geofabrik [3] | gis_osm_transport_a_free_1 | fclass = ’airport’ |
| | CLC [4] | | Code_18=’124’ |
| **Airfields** | Basis-DLM [1] | ver04_f | ART in ('5520', '5540', '5550') AND (ZUS IS NULL or ZUS = 'None') |
| | OSM [2] retrieved from Geofabrik [3] | gis_osm_transport_a_free_1 | fclass = 'airfield' OR fclass = 'apron' |
| **Military** | Basis-DLM [1] | geb03_f | ADF = '4720' |
| **Mining** | Basis-DLM [1] | sie02_f | OBJART ='41005' OR OBJART ='41004' |
| | OSM [2] retrieved from Geofabrik [3] | gis_osm_landuse_a_free_1 | fclass = 'quarry' |
| | CLC [4] | | Code_18='131' |
| **Recreational** | Basis-DLM [1] | sie02_f | OBJART = '41008' |
| **Cemetery** | Basis-DLM [1] | sie02_f | OBJART = '41009' |
| **Birds protected areas (SPA)** | WDPA [8] | | DESIG_ENG = 'Special Protection Area (Birds Directive)' |
| **Nature reserve (NSG)** | WDPA [8] | | DESIG_ENG = ’Nature Reserve’ |
| | Basis-DLM [1] | geb03_f | ADF =’1621’ |
| | OSM [2] retrieved from Geofabrik [3] | gis_osm_landuse_a_free_1 | fclass=’nature_reserve’ |
| **National park** | WDPA [8] | | DESIG_ENG = ’National Park’ |
| | Basis-DLM [1] | geb03_f | ADF =’1670’ |
| **FFH** | WDPA [8] | | Desig='Site of Community Importance (Habitats Directive)' |
| **Biosphere (core zones)** | BFN [9] | Bio_Zonierung2021_3035 | ZONIERUNG = 'Kernzone' |
| **Biosphere (Maintenance zones)** | BFN [9] | Bio_Zonierung2021_3035 | ZONIERUNG = 'Pflegezone' |

| | | | |
|---|---|---|---|
| **Biosphere (Development zones)** | BFN [9] | Bio_Zonierung2021_3035 | ZONIERUNG = 'Entwicklungszone' |
| **Nature park** | BFN [9] | Naturparke2021 | None |
| **Ramsar** | WDPA [8] | | Desig='Ramsar Site, Wetland of International Importance' |
| **Protected landscapes** | WDPA [8] | | DESIG_ENG = 'Landscape Protection Area' |
| **Water protection (I&II)** | BfG [10] | AM_drinkingWaterProtectionArea-DE | WSG_ZONE in ( '1' , '1A', '1B', '2', '2A' , '2a','2b', '2B', '2B1' , '2B2' ,'GW_I', 'GW_II', 'I', 'II', 'IIA', 'IIB', 'IIC', 'qual I', 'qual II', 'TWS I', 'TWS II', 'TWS II/1', 'TWS II/2', 'TWS II/3', 'Zone I', 'Zone II', 'keine Angabe') |
| | LFU-RP [11] | | SCHUTZZO_1 in ( 'Zone I' , 'Zone II' , 'Zone II A' , 'Zone II S' ) |
| | LUBW [12] | | ZONE in ( 'Zone I und II bzw. IIA' , 'Zone IIB' ) |
| **Historical** | OSM [2] retrieved from Geofabrik [3] | gis_osm_pois_a_free_1 | fclass IN ('archaeological','monument','memorial','castle') |
| **Buildings commercial** | Hausumringe [6] | | GFK IN ('31001_2000', '31001_2010', '31001_2020', '31001_2030','31001_2040', '31001_2050', '31001_2051', '31001_2052','31001_2053', '31001_2054', '31001_2055', '31001_2056','31001_2060', '31001_2070', '31001_2071', '31001_2072','31001_2073', '31001_2074', '31001_2080', '31001_2081','31001_2082', '31001_2083', '31001_2090', '31001_2091','31001_2092', '31001_2093', '31001_2094') |
| **Mixed usage** | Basis-DLM [1] | sie02_f | OBJART ='41006' |
| | OSM [2] retrieved from Geofabrik [3] | gis_osm_landuse_a_free_1 | fclass='farmyard' |
| **Slope** | EU-DEM v1.1 [13] | | None |

| | | | |
|---|---|---|---|
| **Birds protected areas (SPA)** | WDPA [8] | | DESIG_ENG = 'Special Protection Area (Birds Directive)' |
| **Nature reserve (NSG)** | WDPA [8] | | Desig='Naturschutzgebiet' |
| **National Park** | WDPA [8] | | Desig='Nationalpark' |
| **Marine protected areas** | WDPA [8] | | Desig='Baltic Sea Protected Area (HELCOM)' OR DESIG='Marine Protected Area (OSPAR)' |
| **Sea depth** | ELC Inspire [14] | | None |
| **Border** | VG250 [15] | VG250_STA | GF = 4 |
| **Sea border** | CONTIS Administration [16] | Boundaries | None |
| | VG250 | VG250_STA | GF !=4 |
| **Offshore Military**** | Raumordnungsplan AWZ [17] | Defence | None |
| | CONTIS Administration [16] | Military_Practice_AreaPolygon | None |
| **Offshore Pipeline** | CONTIS Facility [18] | PipelinesLine | None |
| **Offshore Data Cables** | CONTIS Facility [18] | Data_CablesLine | status = 'inUse' |
| **Offshore HV Cables** | CONTIS Facility [18] | High_Voltage_CablesLine | status != 'Unknown' and status!='OutOfUse' |
| **Offshore Platforms** | CONTIS Facility [18] | PlatformsPoint | status != 'Decommissioned' |
| **Priority Shipping Areas** | Raumordnungsplan AWZ [17] | Shipping | Type = 'priority area' |
| | Niedersachsen LROP 2017 Neubekanntmachung [19] | LROP2017gesamt_Schifffahrt_A | ZVS_Text = 'Vorranggebiet Schifffahrt' |
| | Landesraum-entwicklungsprogramm Mecklenburg-Vorpommern 2016 [20] | Gebiete_fuer_Schifffahrt_LEPMV2016 | festlegung = 'Marines Vorranggebiet Schifffahrt' |
| | Fortschreibung des Landesentwicklungs-plans Schleswig-Holstein 2010 (2. Entwurf 2020) [21] | LEP_SH Entwurf 2020 Teil C Hauptkarte Shapefile vorrang_schifffahrt | None |

**CONTIS Administration for Military in Federal States Sea, ROP for Military in EEZ

## Evaluation of land use data sets (Section 2.2)

**Table 2**
Exclusions for evaluation of land use datasets

| Criterion | Dataset | Buffer |
|---|---|---|
| **Airfields** | variable | 1500 m |
| **Airports** | variable | 6000 m |
| **Forests** | variable | 0 m |
| **Industrial/Commercial** | variable | 2H |
| **Lakes** | variable | 100 m |
| **Mixed used areas** | variable | 2H |
| **Residential areas** | variable | 3H |
| **Rivers** | variable | 100 m |
| **Airfields** | variable | 1500 m |
| **Biosphere (core zones)** | BFN [7] | 300 m |
| **Birds protected areas (SPA)** | WDPA [6] | 300 m |
| **D-VOR** | OSM [2] | 10000 m |
| **FFH** | WDPA [6] | 300 m |
| **National Park** | WDPA [6] | 300 m |
| **Nature reserve (NSG)** | WDPA [6] | 300 m |
| **Protected Landscapes** | WDPA [6] | 0 m |
| **Seismic stations** | BGR [5] | 1000 m |
| **Slope > 17°** | EU-DEM v1.1 [16] | 0 m |
| **VOR** | OSM [2] | 15000 m |

## Onshore wind potential (Section 2.3)

**Table 3**
Onshore wind exclusions (R: Radius, D: Diameter, H: Height)

| Criterion | Dataset | S1 | S2 | S2a | S2b | S3 |
|---|---|---|---|---|---|---|
| **Airfields** | Basis-DLM [1] | individual* | 1500 m | 1500 m | 1500 m | 1500 m |
| **Airports** | Basis-DLM [1] | individual* | 6000 m | 6000 m | 6000 m | 6000 m |
| **Biosphere (core zones)** | BFN [9] | individual* | 0 m | 0 m | 0 m | 500 m |
| **Biosphere (Development zones)** | BFN [9] | individual* | Not excluded | Not excluded | Not excluded | 500 m |
| **Biosphere (Maintenance zones)** | BFN [9] | individual* | Not excluded | Not excluded | Not excluded | 500 m |
| **Birds protected areas (SPA)** | WDPA [8] | individual* | 300 m | 300 m | 300 m | 500 m |

| | | | | | | |
|---|---|---|---|---|---|---|
| **Border** | VG250 [15] | individual* | 100 m | 100 m | 100 m | 100 m |
| **Buildings commercial** | Hausumringe [6] | individual* | 2H | 2H | 2H | 3H |
| **Buildings health treatment** | Hausumringe [6] | individual* | 1000 m | 1000 m | 1000 m | 1000 m |
| **Buildings mixed usage** | Hausumringe [6] | individual* | 3H | 3H | 3H | 3H |
| **Buildings residential** | Hausumringe [6] | individual* | 3H | 3H | 3H | 1000 m |
| **Camping** | Basis-DLM [1] | individual* | 3H | 3H | 3H | 1000 m |
| **Cemetery** | Basis-DLM [1] | individual* | 0 m | 0 m | 0 m | 0 m |
| **D-VOR** | OSM [2] | individual* | 10000 m | 10000 m | 10000 m | 10000 m |
| **Farmland** | Not excluded | Not excluded | Not excluded | Not excluded | Not excluded | Not excluded |
| **FFH** | WDPA [8] | individual* | 300 m | 300 m | 300 m | 500 m |
| **Forests** | Basis-DLM [1] | individual* | Not excluded | Not excluded | 0 m | 0 m |
| **Grassland** | Not excluded | Not excluded | Not excluded | Not excluded | Not excluded | Not excluded |
| **Historical** | OSM [2] | individual* | 1000 m | 1000 m | 1000 m | 1000 m |
| **Industrial/Commercial** | Basis-DLM [1] | individual* | 2H | 2H | 2H | 3H |
| **Inner areas** | Basis-DLM [1] | individual* | 1000 m | 1000 m | 1000 m | 1000 m |
| **Lakes** | Basis-DLM [1] | individual* | 100 m | 100 m | 100 m | 100 m |
| **Military** | Basis-DLM [1] | individual* | 0 m | 0 m | 0 m | 0 m |
| **Mineral extraction** | Basis-DLM [1] | individual* | 0 m | 0 m | 0 m | 0 m |
| **Mixed usage** | Basis-DLM [1] | individual* | 2H | 2H | 2H | 3H |
| **Motorway** | Basis-DLM [1] | individual* | 40 + R | 40 + R | 40 + R | 40 + R |
| **National park** | WDPA [8] | individual* | 300 m | 300 m | 300 m | 500 m |
| **Nature park** | BFN [9] | individual* | Not excluded | Not excluded | Not excluded | 0 m |
| **Nature reserve (NSG)** | WDPA [8] | individual* | 300 m | 300 m | 300 m | 500 m |

| | | | | | | |
|---|---|---|---|---|---|---|
| **Outer areas** | Basis-DLM [1] | individual* | 3H | 3H | 3H | 1000 m |
| **Power lines** | Basis-DLM [1] | individual* | 100 + D | 100 + D | 100 + D | 100 + D |
| **Primary roads** | Basis-DLM [1] | individual* | 20 + R | 20 + R | 20 + R | 20 + R |
| **Protected landscapes** | WDPA [8] | individual* | Not excluded | 0 m | Not excluded | 0 m |
| **Railways** | Basis-DLM [1] | individual* | 100 + D | 100 + D | 100 + D | 100 + D |
| **Ramsar** | WDPA [8] | individual* | Not excluded | Not excluded | Not excluded | 0 m |
| **Recreational** | Basis-DLM [1] | individual* | 0 m | 0 m | 0 m | 0 m |
| **Regional roads** | Basis-DLM [1] | individual* | R | R | R | R |
| **Rivers** | Basis-DLM [1] | individual* | 100 m | 100 m | 100 m | 100 m |
| **Secondary roads** | Basis-DLM [1] | individual* | R | R | R | R |
| **Seismic station** | BGR [7] | individual* | 1000 m | 1000 m | 1000 m | 1000 m |
| **Slope >17°** | EU-DEM v1.1 [13] | individual* | 0 m | 0 m | 0 m | 0 m |
| **Stream** | OSM [2] | individual* | 0 m | 0 m | 0 m | 0 m |
| **VOR** | OSM [2] | individual* | 15000 m | 15000 m | 15000 m | 15000 m |
| **Water protection (I&II)** | Processed (s. Table 1) | individual* | 50 m | 50 m | 50 m | 50 m |

* see Table 4

**Table 4**
Exclusions for scenario 1

| Criterion | Dataset | SH | HH | NI | HB | NW | HE |
|---|---|---|---|---|---|---|---|
| **Airfields** | Basis-DLM [1] | 1750 m | 1750 m | 1750 m | 1750 m | 1750 m | 1750 m |
| **Airports** | Basis-DLM [1] | 6000 m | 6000 m | 6000 m | 6000 m | 6000 m | 6000 m |
| **Biosphere (core zones)** | BFN [9] | 0 m | 0 m | 0 m | 0 m | 0 m | 0 m |
| **Biosphere (Development zones)** | BFN [9] | Not excl. | Not excl. | 0 m | Not excl. | Not excl. | Not excl. |

| | | | | | | | |
|---|---|---|---|---|---|---|---|
| **Biosphere (Maintenance zones)** | BFN [9] | Not excl. | Not excl. | 0 m | Not excl. | Not excl. | 0 m |
| **Birds protected areas (SPA)** | WDPA [8] | 300+R | 300 m | Not excl. | Not excl. | 300 m | Not excl. |
| **Border** | VG250 [15] | 100 m | 100 m | 100 m | 100 m | 100 m | 100 m |
| **Buildings health treatment** | Hausumringe [6] | 3H | 3H | 3H | 3H | 3H | 1000 m |
| **Buildings mixed usage** | Hausumringe [6] | 3H | 3H | 3H | 3H | 1000 m | 1000 m |
| **Buildings residential** | Hausumringe [6] | 3H | 3H | 3H | 3H | 1000 m | 1000 m |
| **Camping** | Basis-DLM [1] | 3H | 3H | 3H | 3H | 3H | 3H |
| **Cemetery** | Basis-DLM [1] | 0 m | 0 m | 0 m | 0 m | 0 m | 0 m |
| **D-VOR** | OSM [2] | 10000 m | 10000 m | 10000 m | 10000 m | 10000 m | 10000 m |
| **Farmland** | Not excl. | Not excl. | Not excl. | Not excl. | Not excl. | Not excl. | Not excl. |
| **FFH** | WDPA [8] | 200+R | 200 m | Not excl. | Not excl. | 300 m | Not excl. |
| **Forests** | Basis-DLM [1] | 0 m | 0 m | 0 m | 0 m | Not excl. | Not excl. |
| **Grassland** | Not excl. | Not excl. | Not excl. | Not excl. | Not excl. | Not excl. | Not excl. |
| **Historical** | OSM [2] | 0 m | 0 m | 0 m | 0 m | 0 m | 0 m |
| **Industrial/Commercial** | Basis-DLM [1] | 2H | 2H | 2H | 2H | 2H | 1000 m |
| **Inner areas** | Basis-DLM [1] | 800 m | 3H | 3H | 3H | 1000 m | 1000 m |
| **Lakes** | Basis-DLM [1] | 50 m | 50 m | 50 m | 50 m | 50 m | 50 m |
| **Military** | Basis-DLM [1] | 0 m | 0 m | 0 m | 0 m | 0 m | 0 m |
| **Mineral extraction** | Basis-DLM [1] | 0 m | 0 m | 0 m | 0 m | 0 m | 0 m |
| **Motorway** | Basis-DLM [1] | 40+R | 40+R | 40+R | 40+R | 40+R | 40+R |
| **National park** | WDPA [8] | 300+R | 0 m | 0 m | 0 m | 300 m | 0 m |
| **Nature park** | BFN [9] | Not excl. | Not excl. | Not excl. | 0 m | Not excl. | Not excl. |

| | | | | | | | |
|---|---|---|---|---|---|---|---|
| **Nature reserve (NSG)** | WDPA [8] | 200+R | 300 m | 0 m | 0 m | 300 m | 0 m |
| **Outer areas** | Basis-DLM [1] | 3H | 3H | 3H | 3H | 1000 m | 1000 m |
| **Power lines** | Basis-DLM [1] | 2R | 2R | 2R | 2R | 100+2R | 2R |
| **Primary roads** | Basis-DLM [1] | 20+R | 20+R | 20+R | 20+R | 20+R | 20+R |
| **Protected landscapes** | WDPA [8] | Not excl. | Not excl. | Not excl. | 0 m | 0 m | Not excl. |
| **Railways** | Basis-DLM [1] | 2R | 2R | 2R | 2R | 100+2R | 2R |
| **Ramsar** | WDPA [8] | 300+R | 500 m | Not excl. | 0 m | Not excl. | Not excl. |
| **Recreational** | Basis-DLM [1] | 0 m | 0 m | 0 m | 0 m | 0 m | 0 m |
| **Regional roads** | Basis-DLM [1] | R | R | R | R | R | R |
| **Rivers** | Basis-DLM [1] | 50 m | 50 m | 50 m | 50 m | 50 m | 50 m |
| **Secondary roads** | Basis-DLM [1] | R | R | R | R | R | R |
| **Seismic station** | BGR [7] | 1000 m | 1000 m | 1000 m | 1000 m | 1000 m | 1000 m |
| **Slope >17°** | EU-DEM v1.1 [13] | 0 m | 0 m | 0 m | 0 m | 0 m | 0 m |
| **Stream** | OSM [2] | 0 m | 0 m | 0 m | 0 m | 0 m | 0 m |
| **VOR** | OSM [2] | 15000 m | 15000 m | 15000 m | 15000 m | 15000 m | 15000 m |
| **Water protection (I&II)** | Processed (s. Table 1) | 50 m | 50 m | 50 m | 50 m | 50 m | 50 m |

SH=Schleswig-Holstein; HH=Hamburg; NI=Lower Saxony; HB=Bremen; NW=North Rhine Westphalia; HE=Hessen

| **Criterion** | **Dataset** | **RP** | **BW** | **BY** | **SL** | **BE** |
|---|---|---|---|---|---|---|
| **Airfields** | Basis-DLM [1] | 1750 m | 1750 m | 1750 m | 1750 m | 1750 m |
| **Airports** | Basis-DLM [1] | 6000 m | 6000 m | 6000 m | 6000 m | 6000 m |
| **Biosphere (core zones)** | BFN [9] | 0 m | 200 m | 0 m | 0 m | 0 m |

| | | | | | | |
|---|---|---|---|---|---|---|
| **Biosphere (Development zones)** | BFN [9] | Not excl. | Not excl. | Not excl. | Not excl. | Not excl. |
| **Biosphere (Maintenance zones)** | BFN [9] | 0 m | Not excl. | Not excl. | 0 m | Not excl. |
| **Birds protected areas (SPA)** | WDPA [8] | Not excl. | 700 m | 10H | 200 m | Not excl. |
| **Border** | VG250 [15] | 100 m | 100 m | 100 m | 100 m | 100 m |
| **Buildings health treatment** | Hausumringe [6] | 800 m | 3H | 3H | 3H | 3H |
| **Buildings mixed usage** | Hausumringe [6] | 3H | 3H | 3H | 3H | 3H |
| **Buildings residential** | Hausumringe [6] | 3H | 3H | 10H | 3H | 3H |
| **Camping** | Basis-DLM [1] | 3H | 3H | 3H | 3H | 3H |
| **Cemetery** | Basis-DLM [1] | 0 m | 0 m | 0 m | 0 m | 0 m |
| **D-VOR** | OSM [2] | 10000 m | 10000 m | 10000 m | 10000 m | 10000 m |
| **Farmland** | Not excl. | Not excl. | Not excl. | Not excl. | Not excl. | Not excl. |
| **FFH** | WDPA [8] | Not excl. | Not excl. | Not excl. | 200 m | Not excl. |
| **Forests** | Basis-DLM [1] | Not excl. | Not excl. | Not excl. | Not excl. | 0 m |
| **Grassland** | Not excl. | Not excl. | Not excl. | Not excl. | Not excl. | Not excl. |
| **Historical** | OSM [2] | 0 m | 0 m | 0 m | 0 m | 0 m |
| **Industrial/Commercial** | Basis-DLM [1] | 2H | 2H | 2H | 2H | 2H |
| **Inner areas** | Basis-DLM [1] | 1100 m | 3H | 10H | 3H | 3H |
| **Lakes** | Basis-DLM [1] | 50 m | 50 m | 50 m | 50 m | 50 m |
| **Military** | Basis-DLM [1] | 0 m | 0 m | 0 m | 0 m | 0 m |
| **Mineral extraction** | Basis-DLM [1] | 0 m | 0 m | 0 m | 0 m | 0 m |
| **Motorway** | Basis-DLM [1] | 40+R | 40+R | 40+R | 40+R | 40+R |

| | | | | | | |
|---|---|---|---|---|---|---|
| **National park** | WDPA [8] | 0 m | 200 m | 0 m | 0 m | 0 m |
| **Nature park** | BFN [9] | Not excl. | Not excl. | Not excl. | Not excl. | Not excl. |
| **Nature reserve (NSG)** | WDPA [8] | 0 m | 200 m | 0 m | 200 m | 0 m |
| **Outer areas** | Basis-DLM [1] | 3H | 3H | 3H | 3H | 3H |
| **Power lines** | Basis-DLM [1] | 2R | 2R | 2R | 2R | 2R |
| **Primary roads** | Basis-DLM [1] | 20+R | 20+R | 20+R | 20+R | 20+R |
| **Protected landscapes** | WDPA [8] | Not excl. | Not excl. | Not excl. | Not excl. | Not excl. |
| **Railways** | Basis-DLM [1] | 2R | 2R | 2R | 2R | 2R |
| **Ramsar** | WDPA [8] | Not excl. | Not excl. | Not excl. | 0 m | Not excl. |
| **Recreational** | Basis-DLM [1] | 800 m | 0 m | 0 m | 0 m | 0 m |
| **Regional roads** | Basis-DLM [1] | R | R | R | R | R |
| **Rivers** | Basis-DLM [1] | 50 m | 50 m | 50 m | 50 m | 50 m |
| **Secondary roads** | Basis-DLM [1] | R | R | R | R | R |
| **Seismic station** | BGR [7] | 1000 m | 1000 m | 1000 m | 1000 m | 1000 m |
| **Slope >17°** | EU-DEM v1.1 [13] | 0 m | 0 m | 0 m | 0 m | 0 m |
| **Stream** | OSM [2] | 0 m | 0 m | 0 m | 0 m | 0 m |
| **VOR** | OSM [2] | 15000 m | 15000 m | 15000 m | 15000 m | 15000 m |
| **Water protection (I&II)** | Processed (s. Table 1) | 50 m | 50 m | 50 m | 50 m | 50 m |

RP=Rhineland Palatinate; BW=Baden Wurttemberg; BY=Bavaria; SL=Saarland; BE=Berlin;

| **Criterion** | **Dataset** | **BB** | **MV** | **SN** | **ST** | **TH** |
|---|---|---|---|---|---|---|
| **Airfields** | Basis-DLM [1] | 1750 m | 1750 m | 1750 m | 1750 m | 1750 m |
| **Airports** | Basis-DLM [1] | 6000 m | 6000 m | 6000 m | 6000 m | 6000 m |

| | | | | | | |
|---|---|---|---|---|---|---|
| **Biosphere (core zones)** | BFN [9] | 0 m | 500 m | 0 m | 1000 m | 0 m |
| **Biosphere (Development zones)** | BFN [9] | Not excl. | 500 m | Not excl. | 1000 m | 0 m |
| **Biosphere (Maintenance zones)** | BFN [9] | Not excl. | 500 m | Not excl. | 1000 m | 0 m |
| **Birds protected areas (SPA)** | WDPA [8] | Not excl. | 500 m | Not excl. | Not excl. | Not excl. |
| **Border** | VG250 [15] | 100 m | 100 m | 100 m | 100 m | 100 m |
| **Buildings health treatment** | Hausumringe [6] | 3H | 1000 m | 3H | 1200 m | 3H |
| **Buildings mixed usage** | Hausumringe [6] | 3H | 800 m | 3H | 3H | 3H |
| **Buildings residential** | Hausumringe [6] | 3H | 800 m | 3H | 3H | 3H |
| **Camping** | Basis-DLM [1] | 3H | 3H | 3H | 3H | 3H |
| **Cemetery** | Basis-DLM [1] | 0 m | 0 m | 0 m | 0 m | 0 m |
| **D-VOR** | OSM [2] | 10000 m | 10000 m | 10000 m | 10000 m | 10000 m |
| **Farmland** | Not excl. | Not excl. | Not excl. | Not excl. | Not excl. | Not excl. |
| **FFH** | WDPA [8] | Not excl. | 500 m | Not excl. | Not excl. | Not excl. |
| **Forests** | Basis-DLM [1] | Not excl. | 0 m | 0 m | 0 m | 0 m |
| **Grassland** | Not excl. | Not excl. | Not excl. | Not excl. | Not excl. | Not excl. |
| **Historical** | OSM [2] | 0 m | 1000 m | 1000 m | 0 m | 0 m |
| **Industrial/Commercial** | Basis-DLM [1] | 2H | 2H | 2H | 2H | 2H |
| **Inner areas** | Basis-DLM [1] | 1000 m | 1000 m | 3H | 1000 m | 1000 m |
| **Lakes** | Basis-DLM [1] | 50 m | 50 m | 50 m | 50 m | 50 m |
| **Military** | Basis-DLM [1] | 0 m | 0 m | 0 m | 0 m | 0 m |
| **Mineral extraction** | Basis-DLM [1] | 0 m | 0 m | 0 m | 0 m | 0 m |

| | | | | | | |
|---|---|---|---|---|---|---|
| **Motorway** | Basis-DLM [1] | 40+R | 40+R | 40+R | 40+R | 40+R |
| **National park** | WDPA [8] | 0 m | 1000 m | 0 m | 0 m | 600 m |
| **Nature park** | BFN [9] | Not excl. | 500 m | Not excl. | Not excl. | 0 m |
| **Nature reserve (NSG)** | WDPA [8] | 0 m | 500 m | 0 m | 200 m | 300 m |
| **Outer areas** | Basis-DLM [1] | 3H | 800 m | 3H | 3H | 3H |
| **Power lines** | Basis-DLM [1] | 2R | 2R | 2R | 400 m | 2R |
| **Primary roads** | Basis-DLM [1] | 20+R | 20+R | 20+R | 20+R | 20+R |
| **Protected landscapes** | WDPA [8] | Not excl. | Not excl. | Not excl. | 500 m | Not excl. |
| **Railways** | Basis-DLM [1] | 2R | 2R | 2R | 400 m | 2R |
| **Ramsar** | WDPA [8] | Not excl. | Not excl. | Not excl. | Not excl. | Not excl. |
| **Recreational** | Basis-DLM [1] | 0 m | 1000 m | 0 m | 0 m | 0 m |
| **Regional roads** | Basis-DLM [1] | R | R | R | R | R |
| **Rivers** | Basis-DLM [1] | 50 m | 50 m | 50 m | 50 m | 50 m |
| **Secondary roads** | Basis-DLM [1] | R | R | R | R | R |
| **Seismic station** | BGR [7] | 1000 m | 1000 m | 1000 m | 1000 m | 1000 m |
| **Slope >17°** | EU-DEM v1.1 [13] | 0 m | 0 m | 0 m | 0 m | 0 m |
| **Stream** | OSM [2] | 0 m | 0 m | 0 m | 0 m | 0 m |
| **VOR** | OSM [2] | 15000 m | 15000 m | 15000 m | 15000 m | 15000 m |
| **Water protection (I&II)** | Processed (s. Table 1) | 50 m | 50 m | 50 m | 50 m | 50 m |

BB=Brandenburg; MV=Mecklenburg-West Pomerania; SN=Saxony; ST=Saxony Anhalt; TH=Thuringia

## Offshore wind potential (Section 2.4)

**Table 5**
Pre-selected areas for offshore wind

| Scenario | Dataset | File name | Filter |
|---|---|---|---|
| **S2 Legislation** | Raumordnungsplan AWZ [17] | OffshoreWindEnergy | None |
| | Landesraumentwicklungs-programm Mecklenburg-Vorpommern 2016 [20] | Gebiete_fuer_Windenergieanlagen_LEPMV2016 | None |
| | Niedersachsen LROP 2017 Neubekanntmachung [19] | LROP2017gesamt_windenergie | None |
| **S3 Restrictive Legislation** | Raumordnungsplan AWZ [17] | OffshoreWindEnergy | Type = 'priority area' OR Type = 'conditional priority area' |
| | Landesraumentwicklungs-programm Mecklenburg-Vorpommern 2016 [20] | Gebiete_fuer_Windenergieanlagen_LEPMV2016 | festlegung != 'Marines Vorbehaltsgebiet für Windenergieanlagen' |
| | Niedersachsen LROP 2017 Neubekanntmachung [19] | LROP2017gesamt_windenergie | zvs_text = 'Eignungsgebiet Windenergienutzung' |

**Table 6**
Offshore wind exclusions

| Criterion | Data set | S1 | S1a | S2 | S3 |
|---|---|---|---|---|---|
| **Birds protected areas (SPA)** | WDPA [8] | 0 | 0 | Not excluded | Not excluded |
| **Border** | VG250 [15] | 15000 m | 15.000 m | Not excluded | Not excluded |
| **Data Cables** | CONTIS Facilities [18] | 500 m | 500 m | 500 m | 500 m |
| **HV Cables** | CONTIS Facilities [18] | 500 m | 500 m | 500 m | 500 m |
| **Marine protected areas** | WDPA [8] | 0 | 0 | Not excluded | Not excluded |
| **Military** | Processed (s. Table 1) | 0 | Not excluded | Not excluded | Not excluded |
| **National Park** | WDPA [8] | 0 | 0 | Not excluded | Not excluded |
| **Nature reserve (NSG)** | WDPA [8] | 0 | 0 | Not excluded | Not excluded |
| **Pipeline** | CONTIS Facilities [18] | 500 m | 500 m | 500 m | 500 m |
| **Platforms** | CONTIS Facilities [18] | 500 m | 500 m | 500 m | 500 m |
| **Priority Shipping Areas** | Processed (s. Table 1) | 500 m | 500 m | Not excluded | Not excluded |

| | | | | | |
|---|---|---|---|---|---|
| **Sea border** | Processed (s. Table 1) | 500 m | 500 m | Not excluded | Not excluded |
| **Sea depth** | ELC Inspire [14] | 1000 m | 1000 m | Not excluded | Not excluded |
| **Seismic Stations** | BGR [7] | 1000 m | 1000 m | Not excluded | Not excluded |

## Open-field photovoltaic potential (Section 2.5)

In scenario S1 Side Strips of the open-field photovoltaic potentials, the side stripes along motorways and railways are considered as pre-selected areas. The area of the side strips are defined by extracting the line features from Basis-DLM [1] and buffering these with half of their width. For motorways either the given width of Basis-DLM [1] (key: BRF) is used or a default width of 40 m is assumed. The area of railways is defined with a default width of 10 m.

In scenario S2 and S3 areas with poor soil quality are used as pre-selected ones. These are defined by the overlap of the Soil Quality Data SQR [22] and farmland areas, identified by Basis-DLM [1] (File: veg01_f; Filter: VEG='1010' ). The resulting areas are named "Processed SQR" in the following.

**Table 7**
Pre-selected areas for open-field photovoltaic

| Scenario | Preselected Area | | Dataset | File name | Filter | Distance |
|---|---|---|---|---|---|---|
| **S1 Side Strips** | Railways | Included | Basis-DLM [1] | ver03_l | ZUS != '2100' OR ZUS is null) AND HDU_X = 0 AND BKT='1100' | 200 |
| | | Excluded | Basis-DLM [1] | ver03_l | ZUS != '2100' OR ZUS is null) AND HDU_X = 0 AND BKT='1100' | 15 |
| | Motorway | Included | Basis-DLM [1] | ver01_l | (ZUS != '2100' OR ZUS is null) AND HDU_X = 0 AND WDM = '1301' | 200 |
| | | Excluded | Basis-DLM [1] | ver01_l | (ZUS != '2100' OR ZUS is null) AND HDU_X = 0 and WDM = '1301' | 15 |
| **S2 Poor Soil** | Poor Soil | Included | Processed SQR | | *Values < 30* | |
| **S3 Combination** | Railways | Included | Basis-DLM [1] | ver03_l | ZUS != '2100' OR ZUS is null) AND HDU_X = 0 AND BKT='1100' | 200 |
| | | Excluded | Basis-DLM [1] | ver03_l | ZUS != '2100' OR ZUS is null) AND HDU_X = 0 AND BKT='1100' | 15 |
| | | | Processed SQR | | *Values > 40* | |
| | Motorway | Included | Basis-DLM [1] | ver01_l | (ZUS != '2100' OR ZUS is null) AND HDU_X = 0 AND WDM = '1301' | 200 |

| | | | | | | |
|---|---|---|---|---|---|---|
| | | Excluded | Basis-DLM [1] | ver01_l | (ZUS != '2100' OR ZUS is null) AND HDU_X = 0 and WDM = ’1301’ | 15 |
| | | | Processed SQR | | *Values > 40* | |
| | Poor Soil | Included | Processed SQR | | *Values < 30* | |
| | | Excluded | Basis-DLM [1] | ver03_l | ZUS != '2100' OR ZUS is null) AND HDU_X = 0 AND BKT='1100' | 200 |
| | | | Basis-DLM [1] | ver01_l | (ZUS != '2100' OR ZUS is null) AND HDU_X = 0 AND WDM = ’1301’ | 200 |

**Table 8**
Open-field photovoltaic exclusions

| **Criterion** | **Dataset** | **S1** | **S2** | **S3** |
|---|---|---|---|---|
| **Birds protected areas (SPA)** | WDPA [8] | 0 m | 0 m | 0 m |
| **Border** | VG250 [15] | 100 m | 100 m | 100 m |
| **Buildings all** | Hausumringe [6] | 0 m | 0 m | 0 m |
| **Camping** | Basis-DLM [1] | 10 m | 10 m | 10 m |
| **Cemetery** | Basis-DLM [1] | 0 m | 0 m | 0 m |
| **Farmland** | Basis-DLM [1] and | Not excluded | See Table 7 | See Table 7 |
| **FFH** | WDPA [8] | 0 m | 0 m | 0 m |
| **Forests** | Basis-DLM [1] | 10 m | 10 m | 10 m |
| **Grassland** | Basis-DLM [1] and SQR [22] | Not excluded | 0 m | 0 m |
| **Historical** | OSM [2] | 0 m | 0 m | 0 m |
| **Industrial/Commercial** | Basis-DLM [1] | 0 m | 0 m | 0 m |
| **Inner areas** | Basis-DLM [1] | 0 m | 0 m | 0 m |
| **Lakes** | Basis-DLM [1] | 10 m | 10 m | 10 m |
| **Military** | Basis-DLM [1] | 0 m | 0 m | 0 m |

| | | | | |
|---|---|---|---|---|
| **Mineral extraction** | Basis-DLM [1] | 0 m | 0 m | 0 m |
| **Motorway** | Basis-DLM [1] | See Table 7 | 200 m | See Table 7 |
| **National park** | WDPA [8] | 0 m | 0 m | 0 m |
| **Nature reserve (NSG)** | WDPA [8] | 0 m | 0 m | 0 m |
| **Outer areas** | Basis-DLM [1] | 0 m | 0 m | 0 m |
| **Power lines** | Basis-DLM [1] | 20 m | 20 m | 20 m |
| **Primary roads** | Basis-DLM [1] | 22.5 m | 22.5 m | 22.5 m |
| **Railways** | Basis-DLM [1] | See Table 7 | 200 m | See Table 7 |
| **Recreational** | Basis-DLM [1] | 0 m | 0 m | 0 m |
| **Regional roads** | Basis-DLM [1] | 22.5 m | 22.5 m | 22.5 m |
| **Rivers** | Basis-DLM [1] | 10 m | 10 m | 10 m |
| **Secondary roads** | Basis-DLM [1] | 22.5 m | 22.5 m | 22.5 m |
| **Slope >10°** | EU-DEM v1.1 [13] | 0 m | 0 m | 0 m |
| **Stream** | OSM [2] | 10 m | 10 m | 10 m |
| **Trees** | Basis-DLM [1] | 10 m | 10 m | 10 m |

[1] Geobasisdaten: © GeoBasis-DE / BKG (2021), 'Digitales Basis-Landschaftsmodell (Ebenen) (Basis-DLM)'. 2021.
[2] OpenStreetMap contributors, 'OpenStreetMap', 2017. https://www.openstreetmap.org (accessed Nov. 12, 2020).
[3] Geofabrik GmbH, 'OpenStreetMap Data Extracts', 2022. http://download.geofabrik.de/
[4] Copernicus Programme, 'CORINE Land Cover (CLC)'. 2018. Accessed: Jun. 13, 2021. [Online]. Available: https://land.copernicus.eu/pan-european/corine-land-cover
[5] Overpass Contributors, 'Overpass Turbo', 2022. https://overpass-turbo.eu/
[6] Geobasisdaten: © GeoBasis-DE / BKG (2021), 'Amtliche Hausumringe Deutschland (HU-DE)'. 2021.
[7] Bundesanstalt für Geowissenschaften und Rohstoffe (BGR), 'Informationen zu deutschen Seismometer-Stationen'. [Online]. Available: https://www.bgr.bund.de/DE/Themen/Erdbeben-Gefaehrdungsanalysen/Seismologie/Seismologie/Seismometer_Stationen/Stationsinfos/d_stationen_node.html
[8] UNEP-WCMC, IUCN, 'The world database on protected areas'. 2016. Accessed: Oct. 22, 2021. [Online]. Available: https://www.protectedplanet.net/
[9] © Bundesamt für Naturschutz (2021), 'BfN-Datensatz'. 2021.
[10] © WasserBLIcK/BfG und Zuständige Behörden der Länder, 2020, 'BfG-Datensatz'. 2020. [Online]. Available: https://www.geoportal.de/Metadata/52d1b6ab-31c7-491b-96c8-be22a31d7313
[11] © Landesamt für Umwelt Rheinland-Pfalz, 'Landesamt für Umwelt Rheinland-Pfalz - Wasserschutz'. 2021.
[12] © Landesanstalt für Umwelt Baden-Württemberg (LUBW), 'Daten- und Kartendienst der LUBW - Wasserschutzgebiete'. 2021. [Online]. Available: https://udo.lubw.baden-wuerttemberg.de/public/index.xhtml
[13] Copernicus Programme, 'European Digital Elevation Model (EU-DEM v1.1)'. 2016. [Online]. Available: https://land.copernicus.eu/imagery-in-situ/eu-dem/eu-dem-v1.1
[14] Bundesamt für Seeschifffahrt und Hydrographie, 'Höhe (Bathymetrie) - INSPIRE-Download-Service'. Jun. 27, 2021. Accessed: Nov. 22, 2021. [Online]. Available: https://www.geoseaportal.de/csw/record/6fe1bb6a-c915-45fe-b84c-d88e4aec55c1
[15] Geobasisdaten: © GeoBasis-DE / BKG (2020), 'Verwaltungsgebiete 1:250 000 (VG250)'. 2020. Accessed: Jul. 05, 2021. [Online]. Available: https://gdz.bkg.bund.de/index.php/default/verwaltungsgebiete-1-250-000-ebenen-stand-01-01-vg250-ebenen-01-01.html
[16] Bundesamt für Seeschifffahrt und Hydrographie, 'CONTIS Administration - WMS'. Jan. 01, 2019. [Online]. Available: https://www.geoseaportal.de/wss/service/CONTIS_Administration/guest?SERVICE=WMS&REQUEST=GetCapabilities&VERSION=1.3.0
[17] Bundesamt für Seeschifffahrt und Hydrographie, 'Raumordnungsplan AWZ – WMS'. Sep. 01, 2021. Accessed: Sep. 01, 2021. [Online]. Available: https://www.geoseaportal.de/mapapps/resources/apps/meeresnutzung/index.html?lang=de
[18] Bundesamt für Seeschifffahrt und Hydrographie, 'CONTIS Facilities'. 2020. Accessed: Nov. 08, 2021. [Online]. Available: https://gdiwiki.bsh.de/wiki/index.php/CONTIS_Facilities
[19] Niedersächsisches Ministerium für Ernährung, Landwirtschaft und Vebraucherschutz, 'Neubekanntmachung der LROP-Verordnung 2017'. 2017. [Online]. Available: https://www.ml.niedersachsen.de/startseite/themen/raumordnung_landesplanung/landesraumordnungsprogramm/datenabgabe_lrop_2017/neubekanntmachung-der-lrop-verordnung-2017-158625.html
[20] Ministerium für Energie, Infrastruktur und Digitalisierung, 'Landesraumentwicklungsprogramm Mecklenburg-Vorpommern 2016 (LEP M-V 2016)'. 2016. Accessed: Sep. 21, 2021. [Online]. Available: https://www.regierung-mv.de/Landesregierung/em/Raumordnung/Landesraumentwicklungsprogramm/aktuelles-Programm/
[21] Landesplanung Schleswig-Holstein/MILIG, 'Fortschreibung des Landesentwicklungsplans Schleswig-Holstein 2010 (2. Entwurf 2020)'. 2021. Accessed: Sep. 20, 2021. [Online]. Available: https://www.bolapla-sh.de/verfahren/bf4796a7-f729-11ea-a85e-0050569710bc/public/detail#procedureDetailsDocumentlist
[22] 'Ackerbauliches Ertragspotenzial der Böden in Deutschland 1:1.000.000. Datenquelle: SQR1000 V1.0'. 2013.
